# Supplementary material for: Emission-frequency separated high quality single-photon sources enabled by phonons
Source: arXiv:1902.06132 ancillary file (2019-07-05)
Supplement: Supplementary file 1 [file supplement.pdf]

# Supplement: Emission-frequency separated high quality single-photon sources enabled by phonons

M. Cosacchi,[1] F. Ungar,[1] M. Cygorek,[2] A. Vagov,[1,3] and V. M. Axt[1]
[1] *Theoretische Physik III, Universität Bayreuth, 95440 Bayreuth, Germany*
[2] *Department of Physics, University of Ottawa, Ottawa, Ontario, Canada K1N 6N5*
[3] *ITMO University, St. Petersburg, 197101, Russia*

## MODEL AND NUMERICAL METHOD

In this supplement we specify in detail the model used in the main paper and outline the numerical procedure used for our simulations. We represent the quantum dot (QD)-cavity system by a Hamiltonian comprising three parts:

$$H = H_{\mathrm{DL}} + H_C + H_{\mathrm{Ph}}, \tag{1}$$

where $H_{\mathrm{DL}}$ describes the QD driven by an external laser, $H_C$ accounts for the coupling of the QD to a quantized cavity mode, while $H_{\mathrm{Ph}}$ represent the interaction with a continuum of longitudinal acoustic (LA) phonons.

Within the usual dipole and rotating wave approximations, the dot-laser Hamiltonian takes the form

$$H_{\mathrm{DL}} = -\hbar\Delta\omega_{\mathrm{LX}}|X\rangle\langle X| - \frac{\hbar}{2}f(t)\left(|X\rangle\langle G| + |G\rangle\langle X|\right) \tag{2}$$

in a frame co-rotating with the laser frequency $\omega_{\mathrm{L}}$. Here, $|G\rangle$ denotes the QD ground state and $|X\rangle$ is the exciton state and a detuning between the laser and exciton frequency $\Delta\omega_{\mathrm{LX}} := \omega_{\mathrm{L}} - \omega_{\mathrm{X}}$ is introduced. $\mathbf{d}$ is the transition dipole and $\mathbf{E}(t)$ the laser field, such that $-\mathbf{d}\cdot\mathbf{E}(t) = -\hbar f(t)/2\,\exp\left(-i\omega_{\mathrm{L}}t\right)$, where $f(t)$ denotes the real envelope function of the exciting laser. $f(t)$ is taken to be a pulse train consisting of Gaussian functions, where each Gaussian has an area $\Theta$ and a pulse length measured by the full-width-at-half-maximum (FWHM). Every $T_{\mathrm{Pulse}}$ the maximum of a Gaussian hits the QD. The dot is coupled to a single-mode microcavity via

$$H_{\mathrm{C}} = \hbar\Delta\omega_{\mathrm{CL}}a^\dagger a + \hbar g\left(a^\dagger|G\rangle\langle X| + a|X\rangle\langle G|\right)\,. \tag{3}$$

The single-mode photons of the cavity are created (annihilated) by the bosonic operator $a^\dagger$ ($a$) and are detuned by $\Delta\omega_{\mathrm{CL}} := \omega_{\mathrm{C}} - \omega_{\mathrm{L}}$ with respect to the laser frequency. The coupling strength between the QD and the microcavity is denoted by $\hbar g$. Furthermore, the pure dephasing-type coupling [1–3] between the QD and a continuum of longitudinal acoustic (LA) phonons is modeled as

$$H_{\mathrm{Ph}} = \hbar\sum_{\mathbf{q}}\omega_{\mathbf{q}}b^\dagger_{\mathbf{q}}b_{\mathbf{q}} + \hbar\sum_{\mathbf{q}}\left(\gamma^{\mathrm{X}}_{\mathbf{q}}b^\dagger_{\mathbf{q}} + \gamma^{\mathrm{X}*}_{\mathbf{q}}b_{\mathbf{q}}\right)|X\rangle\langle X|\,, \tag{4}$$

where the bosonic operator $b^\dagger_{\mathbf{q}}$ ($b_{\mathbf{q}}$) creates (destroys) phonons with frequency $\omega_{\mathbf{q}}$. $\gamma^{\mathrm{X}}_{\mathbf{q}}$ denotes the deformation-potential-type coupling constant between the exciton state and the $\mathbf{q}$-th bosonic mode, which is obtained as the difference between the electron-phonon and hole-phonon constants, $\gamma^{\mathrm{X}}_{\mathbf{q}} = \gamma^{\mathrm{e}}_{\mathbf{q}} - \gamma^{\mathrm{h}}_{\mathbf{q}}$. We consider bulk-phonon modes with linear dispersion, $\omega_{\mathbf{q}} = v_s|\mathbf{q}|$, with the sound velocity $v_s$. With these assumptions the coupling constants take on the form

$$\gamma^{\mathrm{e(h)}}_{\mathbf{q}} = \Psi^{\mathrm{e(h)}}(\mathbf{q})\frac{|\mathbf{q}|D_{\mathrm{e(h)}}}{\sqrt{2V\rho\hbar\omega_{\mathbf{q}}}}\,, \tag{5}$$

where $\rho$ is the density of the material, $V$ the sample volume, $D_{\mathrm{e(h)}}$ the deformation potential constant, and $\Psi^{\mathrm{e(h)}}(\mathbf{q})$ the form factor that is obtained as the Fourier transform of the absolute square of the confined carrier wave functions. The coupling constant enters the phonon spectral density

$$J(\omega) = \sum_{\mathbf{q}}\left|\gamma^{\mathrm{X}}_{\mathbf{q}}\right|^2\,\delta(\omega - \omega_{\mathbf{q}})\,, \tag{6}$$

which in turn determines the depth of the phonon-induced memory [4]. Assuming a spherical dot with harmonic confinement yields

$$J(\omega) = \frac{\omega^3}{4\pi^2\rho\hbar v_s^5}\left\{D_{\mathrm{e}}\exp\left(-\frac{\omega^2a_{\mathrm{e}}^2}{4v_s^2}\right) - D_{\mathrm{h}}\exp\left(-\frac{\omega^2a_{\mathrm{h}}^2}{4v_s^2}\right)\right\}^2\,, \tag{7}$$

where $a_{\mathrm{e(h)}}$ denotes the electron (hole) confinement length.

For the calculations in the main text, we use values that are typical for GaAs self-assembled QDs [5]: $D_{\mathrm{e}} = 7.0\,\mathrm{eV}$, $D_{\mathrm{h}} = -3.5\,\mathrm{eV}$, $\rho = 5370\,\mathrm{kg/m^3}$, $v_s = 5110\,\mathrm{m/s}$, $a_{\mathrm{e}}/a_{\mathrm{h}} = 1.15$. This leaves only the dot diameter as a free parameter in the shape of the electron confinement length, i.e., $6\,\mathrm{nm} = 2a_{\mathrm{e}}$, as quoted in the main text.

Finally, radiative decay of the QD exciton as well as cavity losses are included via Lindblad-type superoperators $\mathcal{L}_{|G\rangle\langle X|,\gamma}\bullet$ and $\mathcal{L}_{a,\kappa}\bullet$, respectively, with

$$\mathcal{L}_{O,\Gamma}\bullet = \Gamma\left(O\bullet O^\dagger - \frac{1}{2}\left\{\bullet, O^\dagger O\right\}_+\right). \tag{8}$$

Here, $\{\cdot,\cdot\}_+$ denotes the anti-commutator, $O$ is a system operator, and $\Gamma$ the decay rate of the associated loss process.

We solve the Liouville-von Neumann equation

$$\dot{\rho} = -\frac{i}{\hbar}\{H,\rho\}_- + \mathcal{L}\rho \tag{9}$$

with $H = H_{\mathrm{DL}} + H_C + H_{\mathrm{Ph}}$ and $\mathcal{L}\bullet = \mathcal{L}_{|G\rangle\langle X|,\gamma}\bullet + \mathcal{L}_{a,\kappa}\bullet$, where $\{\cdot,\cdot\}_-$ is the commutator. The density matrix $\rho$ is assumed to initially factorize into a subsystem part corresponding to the dot-cavity system (DL+C) and a phonon part (Ph). The phonon part is initially taken to be a thermal distribution. We employ an iterative real-time path integral method [6, 7] to obtain the time-dependent reduced density matrix $\bar{\rho} = \mathrm{Tr}_{\mathrm{Ph}}[\rho]$. To the best of our knowledge this method is so far the only one where accounting for the influence of the infinitely many LA phonon modes has been realized in a numerically complete way, i.e., without any further approximations to the model described above, since all phonon contributions can be integrated out analytically. Furthermore, recent developments within this formalism allow for the consistent and natural inclusion of Lindblad-type losses [8] and the consideration of more subsystem levels beyond the few-level limit due to an exact reformulation of the iterative scheme [9]. In fact, the reformulation presented in the supplement of Ref. [9] reduces the numerical demand in our present application by many orders of magnitude without which the simulations presented in the main text would have been impossible. Finally, the two-time photonic correlation function $G^{(2)}(t,\tau) = \langle a^\dagger(t)a^\dagger(t+\tau)a(t+\tau)a(t)\rangle$ necessary for the calculation of the single-photon purity is obtained following a numerically complete algorithm that has been proposed recently [10]. In particular, this algorithm avoids the quantum regression theorem, which is valid only when all bath interactions are Markovian [11]. Indeed, it is known that the coupling to LA phonons induces a memory of several picoseconds [4] and thus a Markovian treatment of the QD-phonon interaction would not be adequate.

[1] L. Besombes, K. Kheng, L. Marsal, and H. Mariette, Phys. Rev. B **63**, 155307 (2001).
[2] P. Borri, W. Langbein, S. Schneider, U. Woggon, R. L. Sellin, D. Ouyang, and D. Bimberg, Phys. Rev. Lett. **87**, 157401 (2001).
[3] B. Krummheuer, V. M. Axt, and T. Kuhn, Phys. Rev. B **65**, 195313 (2002).
[4] A. Vagov, M. D. Croitoru, M. Glässl, V. M. Axt, and T. Kuhn, Phys. Rev. B **83**, 094303 (2011).
[5] B. Krummheuer, V. M. Axt, T. Kuhn, I. D'Amico, and F. Rossi, Phys. Rev. B **71**, 235329 (2005).
[6] N. Makri and D. E. Makarov, The J. Chem. Phys. **102**, 4600 (1995).
[7] N. Makri and D. E. Makarov, The J. Chem. Phys. **102**, 4611 (1995).
[8] A. M. Barth, A. Vagov, and V. M. Axt, Phys. Rev. B **94**, 125439 (2016).
[9] M. Cygorek, A. M. Barth, F. Ungar, A. Vagov, and V. M. Axt, Phys. Rev. B **96**, 201201(R) (2017).
[10] M. Cosacchi, M. Cygorek, F. Ungar, A. M. Barth, A. Vagov, and V. M. Axt, Phys. Rev. B **98**, 125302 (2018).
[11] D. P. S. McCutcheon, Phys. Rev. A **93**, 022119 (2016).
